# Supplementary material for: From Accurate Quantum Chemistry to Converged Thermodynamics for Ion Pairing in Solution
Source: arXiv:2603.06800 source file (2026-11-11)
Supplement: Supplementary file 3 [file ca_water_structural_summary.tex]

\begin{table}[htbp]
\centering
\caption{Calcium hydration properties from simulations at different electronic-structure levels. Coordination-number uncertainties are equilibrium distribution standard deviations. Ca--O distance and residence-time uncertainties are standard errors from five contiguous trajectory blocks. Residence times use the Direct/Hofer definition with a 0.5~ps persistence criterion.}
\label{tab:ca_water_structural_summary}
\begin{tabular}{lccc}
\toprule
Method & CN & $\langle r_{\mathrm{Ca-O}}\rangle$ / $\mathrm{\AA}$ & $\tau_{\mathrm{Direct}}$ / ps \\
\midrule
revPBE-D3 & $6.7 \pm 0.5$ & $2.454 \pm 0.003$ & $19.83 \pm 0.43$ \\
revPBE0-D3 & $7.3 \pm 0.4$ & $2.517 \pm 0.001$ & $22.70 \pm 0.79$ \\
RPA & $8.1 \pm 0.3$ & $2.532 \pm 0.002$ & $29.17 \pm 1.35$ \\
MP2 & $7.6 \pm 0.5$ & $2.527 \pm 0.001$ & $25.24 \pm 0.63$ \\
CCSD(T) & $7.7 \pm 0.4$ & $2.537 \pm 0.002$ & $25.97 \pm 3.44$ \\
\bottomrule
\end{tabular}
\end{table}
