# Supplementary material for: From Accurate Quantum Chemistry to Converged Thermodynamics for Ion Pairing in Solution
Source: arXiv:2603.06800 source file (2026-11-11)
Supplement: Supplementary file 4 [file co3_water_structural_summary.tex]

\begin{table}[htbp]
\centering
\caption{Carbonate hydration properties from simulations at different electronic-structure levels. The coordination number is the smooth OPES-reweighted carbonate--water CN. Distances are between the carbonate carbon and first-shell water oxygens. Carbonate oxygens are excluded from the water selection. Distance and residence uncertainties are standard errors from five contiguous trajectory blocks.}
\label{tab:co3_water_structural_summary}
\begin{tabular}{lccc}
\toprule
Method & CN & $\langle r_{\mathrm{C_{CO_3}-O_w}}\rangle$ / $\mathrm{\AA}$ & $\tau_{\mathrm{Direct}}$ / ps \\
\midrule
revPBE-D3 & $9.5 \pm 0.7$ & $3.581 \pm 0.002$ & $2.01 \pm 0.06$ \\
revPBE0-D3 & $9.1 \pm 0.7$ & $3.558 \pm 0.004$ & $2.68 \pm 0.10$ \\
RPA & $10.6 \pm 0.7$ & $3.544 \pm 0.003$ & $2.28 \pm 0.05$ \\
MP2 & $9.8 \pm 0.7$ & $3.532 \pm 0.006$ & $3.01 \pm 0.15$ \\
CCSD(T) & $9.9 \pm 0.7$ & $3.544 \pm 0.003$ & $2.65 \pm 0.08$ \\
\bottomrule
\end{tabular}
\end{table}
